# Supplementary material for: A new method for flow-based network intrusion detection using the inverse Potts model
Source: arXiv:1910.07266 ancillary file (2021-09-23)
Supplement: Supplementary file 1 [file EFC__Supplementary_Information.pdf]

## Supplementary Information

# A new method for flow-based network intrusion detection using the inverse Potts model

Camila Pontes, Manuela Souza, João Gondim, Matt Bishop and Marcelo Marotta

### APPENDIX A

This appendix contains supplementary information regarding the classifications tests performed on dataset CIDD-001. Table XI shows the classes used for feature discretization. Within CIDD-001 dataset, TCP Flags is the discrete feature with more possible values (32 possibilities), so the alphabet size  $Q$  was set to 32. Each continuous feature values were clustered in a certain number of classes (or bins), up to  $Q$  classes. Classes were determined in such a way that the number of values within each class was similar for all classes.

Table XI  
CLASSES USED FOR FEATURE DISCRETIZATION

| Feature         | List of classes upper limits                                               |
|-----------------|----------------------------------------------------------------------------|
| Duration        | 0.001, 0.002, 0.003, 0.004, 0.005, 0.006, 0.01, 0.04, 1, 10, 100, $\infty$ |
| Protocol        | TCP, UDP, GRE, ICMP, IGMP                                                  |
| Src Port        | 50, 60, 100, 400, 500, 40000, 60000, $\infty$                              |
| Dst Port        | 50, 60, 100, 400, 500, 40000, 60000, $\infty$                              |
| Num. of Bytes   | 50, 60, 70, 90, 100, 110, 200, 300, 400, 500, 700, 1000, 5000, $\infty$    |
| Num. of Packets | 2, 3, 4, 5, 6, 7, 10, 20, $\infty$                                         |
| TCP Flags       | $\{(f_1, f_2, f_3, f_4, f_5)   f_i \in \{0, 1\}\}$                         |

Table XII shows the composition of two non-redundant sampling pools, which are a subset of CIDD-001 dataset used to construct the test sets considered to evaluate classification performance. The first 100,000 non-redundant flows labeled as *normal* were extracted from week 2 simulated traffic to compose a normal traffic sampling pool. Week 2 was chosen because attacks from different types are more equally distributed on this week than on the other weeks. Also, because we want to focus on incoming traffic classification, malicious traffic labeled as *victim* was not selected to compose the sampling pool. Similarly, a malicious traffic sampling pool was composed. All flows labeled as *pingScan* and *bruteForce* were extracted from within week 2 simulated traffic. In addition, the first 90,000 non-redundant DoS flows and the first 9,000 non-redundant port scan flows were selected to compose this pool. Since flows labeled as *pingScan* and *bruteForce* were rare, all samples with these labels were included in the sampling pool. Regarding external traffic, the first 16,900 non-redundant unknown flows and the first 47,700 non-redundant suspicious flows were extracted from CIDD-001 week 3 external server

C. Pontes, J. Gondim and M. A. Marotta are with the University of Brasilia, Brazil, emails: cftpontes@gmail.com, gondim@unb.br, marcelo.marotta@unb.br;

M. Bishop is with the University of California at Davis, Davis, USA, email: mabishop@ucdavis.edu

traffic. Week 3 was chosen because suspicious and unknown flows are more equally distributed on this week than on the other weeks.

Table XII  
STRUCTURE OF SAMPLING POOL FROM CIDD-001 USED TO COMPOSE THE TRAINING/TEST SETS

| Class             | Simulated (week 2) | External (week 3) |
|-------------------|--------------------|-------------------|
| <i>normal</i>     | 100,000            | 0                 |
| <i>attack</i>     | 100,062            | 0                 |
| <i>unknown</i>    | 0                  | 16,900            |
| <i>suspicious</i> | 0                  | 47,700            |

The composition of the sets used to assess classification performance is shown in Table XIII. First, 5,000 normal flows and 5,000 malicious flows were sampled from the normal traffic pool and the malicious traffic pool, respectively, to compose a test set with 10,000 samples. Since flows labeled as *pingScan* and *bruteForce* were rare, all samples with these labels were included. The performance of different classifiers was assessed over this test set using 10-fold cross validation. Similarly, a set with 5,000 suspicious and 5,000 unknown flows randomly sampled from the suspicious traffic pool and the unknown traffic pool, respectively, was constructed. The performance of different classifiers was assessed over this test set. Dataset undersampling was performed in order to obtain a more homogeneous distribution of the different types of malicious traffic.

Table XIII  
CIDD-001 - FLOWS LABELS WITHIN THE TEST SETS

| Label             | Simulated (week2) | External (week 3) |
|-------------------|-------------------|-------------------|
| <i>normal</i>     | 5,000             | 0                 |
| <i>dos</i>        | 1,919             | 0                 |
| <i>portScan</i>   | 1,919             | 0                 |
| <i>pingScan</i>   | 152               | 0                 |
| <i>bruteForce</i> | 910               | 0                 |
| <i>suspicious</i> | 0                 | 5,000             |
| <i>unknown</i>    | 0                 | 5,000             |
| total             | 10,000            | 10,000            |

### APPENDIX B

This appendix contains supplementary information regarding the classifications tests performed on dataset CICIDS17.

Features within this dataset were discretized in such a way that the number of values within each bin was similar for all bins. This discretization is not shown here because of the high number of features (>50 features) in this dataset.

Table XIV shows the composition of labels within the test sets used in each of the two experiments performed. These test sets were composed with randomly chosen samples within the specified scope of the dataset (*e.g.*, day, type of attack). An effort was made to have the different types of malicious traffic equally represented within the test sets, randomly selecting the same number of samples from each type. In experiment 1, the two test sets contained samples from Friday and from other days (not Friday), respectively. In experiment 2, the two test sets contained samples from Wednesday and from other days (not Wednesday), respectively.

Table XIV  
CICIDS17 - FLOW LABELS WITHIN TEST SETS FOR EACH EXPERIMENT

| Label                   | Experiment 1 |            | Experiment 2 |               |
|-------------------------|--------------|------------|--------------|---------------|
|                         | Friday       | not Friday | Wednesday    | not Wednesday |
| <i>Benign</i>           | 5000         | 2500       | 5000         | 2500          |
| <i>DDoS</i>             | 5000         | 0          | 0            | 1250          |
| <i>PortScan</i>         | 0            | 730        | 0            | 730           |
| <i>Bot</i>              | 0            | 420        | 0            | 420           |
| <i>Infiltration</i>     | 0            | 32         | 0            | 32            |
| <i>Brute force</i>      | 0            | 258        | 0            | 258           |
| <i>SQL injection</i>    | 0            | 18         | 0            | 18            |
| <i>XSS</i>              | 0            | 74         | 0            | 74            |
| <i>FTP Patator</i>      | 0            | 730        | 0            | 730           |
| <i>SSH Patator</i>      | 0            | 238        | 0            | 238           |
| <i>DoS Hulk</i>         | 0            | 870        | 2100         | 0             |
| <i>DoS Golden Eye</i>   | 0            | 870        | 2100         | 0             |
| <i>DoS Slowloris</i>    | 0            | 370        | 370          | 0             |
| <i>DoS Slowhttptest</i> | 0            | 430        | 430          | 0             |
| total                   | 10,000       | 7,540      | 10,000       | 6,250         |

## APPENDIX C

This appendix contains supplementary information regarding the classifications tests performed on dataset CICDDoS19. Features within this dataset were discretized in such a way that the number of values within each bin was similar for all bins. This discretization is not shown here because of the high number of features (>50 features) in this dataset.

Table XV shows the composition of labels within the test sets used in each of the three experiments performed. These test sets were composed with randomly chosen samples within the specified scope of the dataset (*e.g.*, day, type of attack). An effort was made to have the different types of malicious traffic equally represented within the test sets, randomly selecting the same number of samples from each type. In experiment 1, the two test sets contained benign plus malicious samples of type DrDoS NTP, and benign plus malicious samples of types Syn and TFTP (not DrDoS NTP), respectively. In experiment 2, the two test sets contained benign plus malicious samples of type Syn, and benign plus malicious samples of types DrDoS NTP and TFTP (not Syn), respectively. In experiment 3, the two test sets contained benign plus malicious samples of type TFTP,

and benign plus malicious samples of types DrDoS NTP and Syn (not TFTP), respectively.

Table XV  
CICDDoS19 - FLOW LABELS WITHIN TEST SETS FOR EACH EXPERIMENT

| Label                | Experiment 1 |               | Experiment 2 |         | Experiment 3 |          |
|----------------------|--------------|---------------|--------------|---------|--------------|----------|
|                      | DrDoS NTP    | not DrDoS NTP | Syn          | not Syn | TFTP         | not TFTP |
| <i>Benign</i>        | 2500         | 1250          | 2500         | 1250    | 2500         | 1250     |
| <i>DrDoS DNS</i>     | 0            | 0             | 0            | 0       | 0            | 0        |
| <i>DrDoS LDAP</i>    | 0            | 0             | 0            | 0       | 0            | 0        |
| <i>DrDoS MSSQL</i>   | 0            | 0             | 0            | 0       | 0            | 0        |
| <i>DrDoS NetBIOS</i> | 0            | 0             | 0            | 0       | 0            | 0        |
| <i>DrDoS NTP</i>     | 2500         | 0             | 0            | 1250    | 0            | 1250     |
| <i>DrDoS SNMP</i>    | 0            | 0             | 0            | 0       | 0            | 0        |
| <i>DrDoS SSDP</i>    | 0            | 0             | 0            | 0       | 0            | 0        |
| <i>DrDoS UDP</i>     | 0            | 0             | 0            | 0       | 0            | 0        |
| <i>Syn</i>           | 0            | 1250          | 2500         | 0       | 0            | 1250     |
| <i>TFTP</i>          | 0            | 1250          | 0            | 1250    | 2500         | 0        |
| <i>UDP lag</i>       | 0            | 0             | 0            | 0       | 0            | 0        |
| <i>LDAP</i>          | 0            | 0             | 0            | 0       | 0            | 0        |
| <i>NetBIOS</i>       | 0            | 0             | 0            | 0       | 0            | 0        |
| <i>MSSQL</i>         | 0            | 0             | 0            | 0       | 0            | 0        |
| <i>Portmap</i>       | 0            | 0             | 0            | 0       | 0            | 0        |
| <i>UDP</i>           | 0            | 0             | 0            | 0       | 0            | 0        |
| <i>UDPLag</i>        | 0            | 0             | 0            | 0       | 0            | 0        |
| total                | 5,000        | 2,750         | 5,000        | 2,750   | 5,000        | 2,750    |
